# Supplementary material for: Anomalous thermopower oscillations in graphene-InAs nanowire vertical heterostructures
Source: arXiv:2009.08882 source file (2020-12-22)
Supplement: Supplementary file 1 [file Supplementary_Info.pdf]

# Supplementary Information:

## Anomalous thermopower oscillations in graphene probed by a local InAs nanoheater

Richa Mitra<sup>1</sup>, Manas Ranjan Sahu<sup>1</sup>, Aditya Sood<sup>2</sup>, Takashi Taniguchi<sup>3</sup>,  
Kenji Watanabe<sup>3</sup>, Hadas Shtrikman<sup>4</sup>, Subroto Mukerjee<sup>1</sup>, A.K. Sood<sup>1</sup>,  
Anindya Das<sup>1</sup> \*

<sup>1</sup>*Department of Physics, Indian Institute of Science, Bangalore-560012, India.*

<sup>2</sup>*Department of Materials Science and Engineering, Stanford University, Stanford, California 94305, USA*

<sup>3</sup>*National Institute for Materials Science, Namiki 1-1, Ibaraki 305-0044, Japan.*

<sup>4</sup>*Department of Physics, Weizmann Institute of Technology, Israel.*

---

\*anindya@iisc.ac.in

## SI 1. Device fabrication

All the devices used in the thermopower measurements are heterostructures of InAs nanowire (NW) and graphene encapsulated by hexagonal Boron Nitride (hBN). In our experiment, we pass current through the NW which acts like a local heating source and measure the thermoelectric voltage across the graphene. Graphene flakes are exfoliated from bulk graphite crystals using scotch tape and then transferred onto 285 nm thick  $\text{SiO}_2$ , thermally grown over p++ doped Si substrate. hBN flakes are separately obtained following similar exfoliation method. Suitable MLG/BLG flakes are identified under the microscope and encapsulated by hBN flakes using the hot pick up technique [1, 2]. After assembling the graphene stack, we separately pick up the suitable NW from a separate substrate and carefully align it at the centre of the the hBN/graphene/hBN stack. The thickness of the top hBN which separates the NW from the graphene are chosen to be around  $\sim 10 - 12$  nm (Fig. S1 b). After assembling the heterostructures, separate probes for graphene and NWs are fabricated. For graphene, we adhere to the conventional one-dimensional edge contact fabrication [3] technique, whereas for the NWs, ohmic contacts are fabricated following the chemical etching technique [4] where saturated  $(\text{NH}_4)_2\text{S}$  solution is used for removing the native oxide. After contact fabrication, all the samples are characterised at room temperature as well as at  $T=1.5$  K. The backgate response of the MLG and BLG have been presented in Fig. 1b of the main manuscript. The typical resistance of the NWs were around  $\sim 25 - 50$   $k\Omega$ .

As shown in the optical image (Fig. S1 a), most of the devices posses intrinsic structural asymmetry where the NW is not placed exactly at the center of the graphene channel which leads to a non-zero thermopower signal. Non-zero  $V_{TE}$  can also result from the unequal contact resistances of the NW probes leading to asymmetric temperature profile across the center. Fig. S1 b shows the thickness of a top hBN flake to be  $\sim 10$  nm, which separates the graphene channel from the NW.

## SI 2. Data extraction

The measurement schematic of our thermopower technique is shown in Fig. S2 a, where we pass a DC current through the NW ( $I_{SD}$ ) and measure thermopower voltage  $V_{TE}$  across the graphene probe. We apply backgate voltage  $V_{BG}$  in the Si/ $\text{SiO}_2$  substrate to tune the graphene density  $n_G$  and  $V_G$  to tune the NW density. Due to the proximity of the NW to the graphene channel which are separated by a thin hBN ( $\sim 10\text{nm}$ ) layer, passing current through the NW may generate drag voltage due to Coulomb interaction between the two systems. Here we mention the method used to accounting the drag effect and extracting the thermopower signal from the raw data. Fig. S3 a and S4 a show 2D colormap of  $V_{TE}$  with heater current  $I_{SD}$  and  $n_G$  for MLG and BLG devices respectively. The raw signal contains both drag ( $V_D$ ) as well as the thermopower signal ( $V_{TE}$ ). The drag signal (flipping part) flips sign as the direction of the current  $I_{SD}$  is reversed whereas the  $V_{TE}$  (the thermopower) signal remains unchanged upon reversing the current direction. To separate out the drag

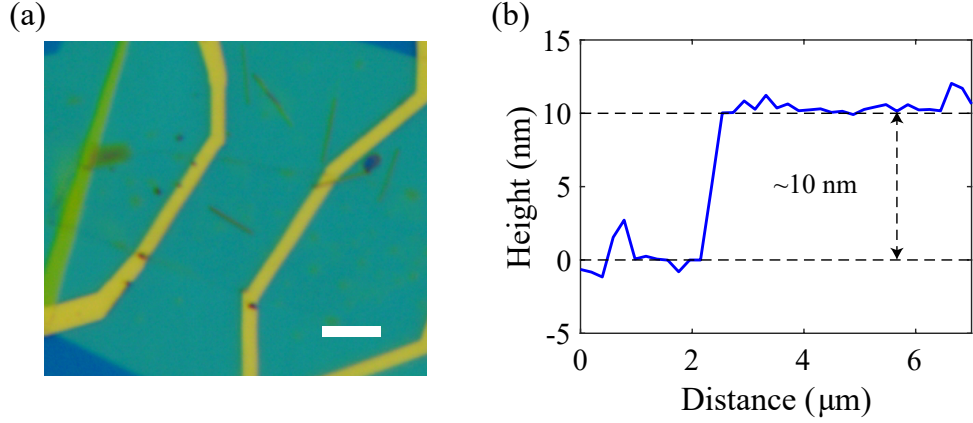

**Figure S1** (a) Optical image of one of the InAs NW-hBN-Graphene-hBN devices having intrinsic asymmetry. The yellow portions are the metal (Cr/Pd/Au) contacts of the encapsulated graphene stack, whereas the NW is placed in the middle of the two graphene contacts. The scale bar is 5  $\mu\text{m}$ . (b) The AFM data showing thickness of the top hBN to be  $\sim 10$  nm. This hBN electrically separates the graphene channel from the NW.

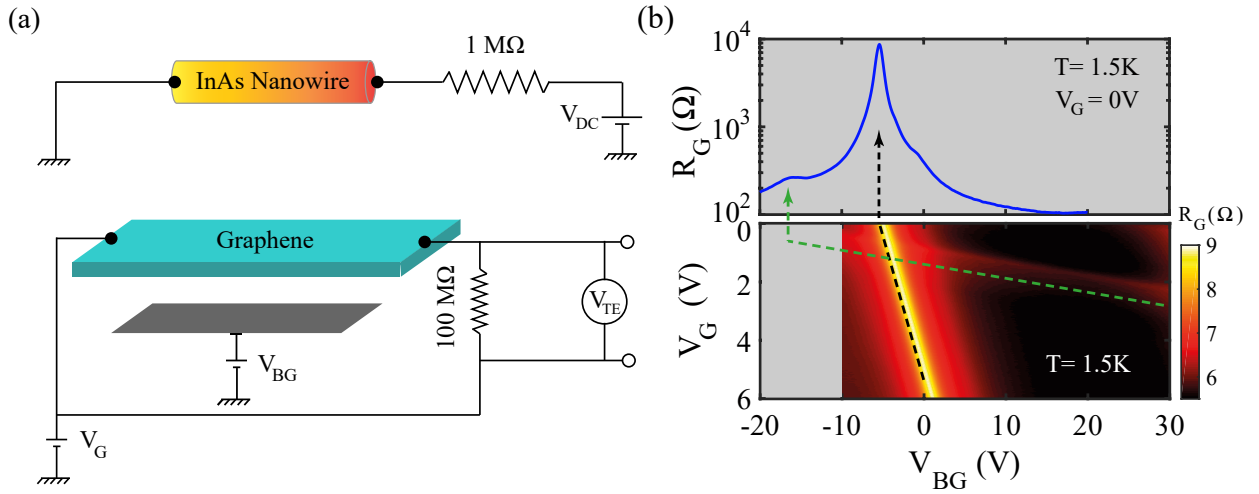

**Figure S2** (a) Thermopower measurement schematic.  $V_{\text{TE}}$  measured in graphene while passing a constant DC current through the NW. (b) (Upper panel) Graphene 2-probe resistance  $R_{\text{G}}$  versus  $V_{\text{BG}}$  plot at  $T=1.5\text{K}$ . (Lower panel) 2D colormap of  $R_{\text{G}}$  versus  $V_{\text{BG}}$  and the graphene gate  $V_{\text{G}}$  measured at  $T=1.5\text{K}$ . The black and the green dashed lines indicate the trajectories of the main Dirac point ( $V_{\text{D1}}$ ) and the additional Dirac point ( $V_{\text{D2}}$ ) with gate voltages, respectively. Arrows in the upper panel indicate that the two Dirac points in the 2D plot originate from  $V_{\text{D1}}$  and  $V_{\text{D2}}$ .

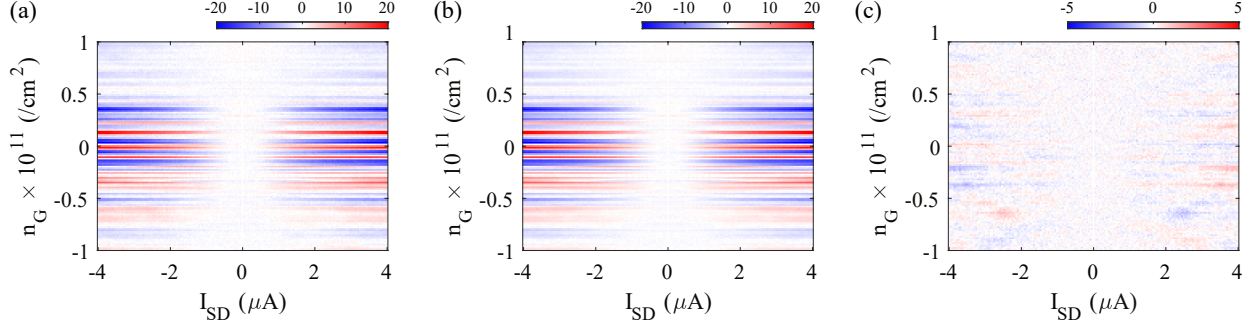

**Figure S3** 2D colormap of  $V_{TE}$  measured in MLG plotted with heating current  $I_{SD}$  and with graphene density  $n_G$  at  $T=1.5K$  and  $B=0T$ . Figure (a), (b) and (c) are the raw signal ( $V_{raw}$ ) and the extracted non-flipping ( $V_{TE}$ ) and the flipping signals ( $V_D$ ) respectively.

effect from the raw signal we adhere to the following method:  $V_D \rightarrow -V_D$ , as  $I_{SD} \rightarrow -I_{SD}$  for drag signals, but the non-flipping part which originates from heating effect ( $\propto I_{SD}^2 R$ ) doesn't change its sign. So, the raw signals can be written as:

$$\begin{aligned} V_{raw}^+ &= V_D + V_{TE} \\ V_{raw}^- &= -V_D + V_{TE} \end{aligned} \quad (1)$$

where  $V_{raw}^+$  and  $V_{raw}^-$  are the raw signals when  $I_{SD}$  is positive and negative, respectively. Combining these two equations, we get:

$$V_{TE} = \frac{1}{2}(V_{raw}^+ + V_{raw}^-) \quad (2)$$

We extracted the  $V_{TE}$  and  $V_D$  according to above equation which are plotted in Figure S3 b and c for the MLG and in S4 b and c for the BLG devices respectively. We observe from these plots that  $V_{TE} \gg V_D$  for both the cases. This is because the NWs used in thermopower experiments usually have higher resistances ( $\sim 25 - 50k\Omega$ ) as compared to our Coulomb drag measurements [5] in another work.

### SI 3. Uneven density profile along the graphene channel

In this section we discuss how the density profile ( $p - n - p$ ) in graphene channel has been interpreted from the experimental data. Figure S2 b (upper panel) shows graphene resistance  $R_G$  plotted with the  $V_{BG}$  where an additional resistive peak appears at  $V_{D2}$  along with the main Dirac point at  $V_{D1}$ . The second resistance peak appears at a negative gate voltage i.e.  $|V_{D2}| > |V_{D1}|$  which indicates that (a) the density profile across the full graphene channel is not uniform, and (b) the region having different density compared to the rest of

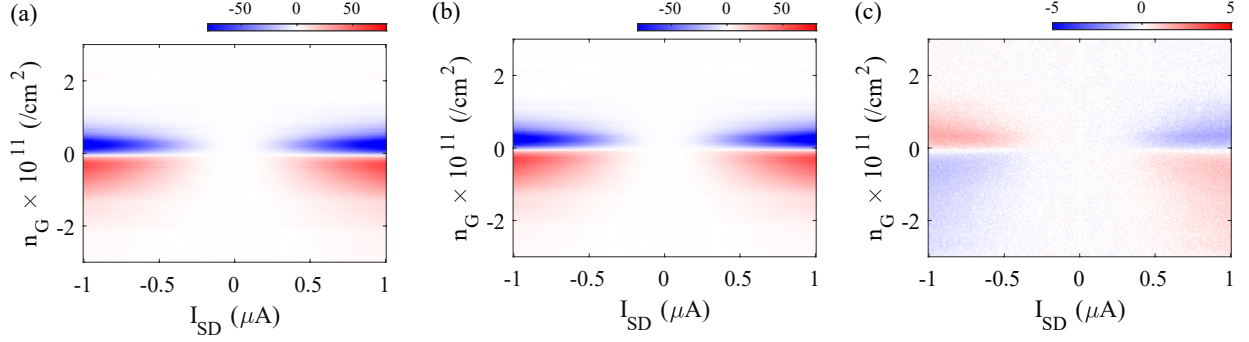

**Figure S4** 2D colormap of  $V_{TE}$  measured in BLG plotted with heating current  $I_{SD}$  and with graphene density  $n_G$  at  $T=1.5K$  and  $B=0T$ . Figure (a), (b) and (c) are the raw signal ( $V_{raw}$ ) and the extracted non-flipping ( $V_{TE}$ ) and the flipping signals ( $V_D$ ) respectively.

the graphene channel is more n-type or electron type. This indicates that along the graphene channel length the effective density profile is  $p - n - p$  type.

To analyse the density profile further, we measure  $R_G$  as a function of both  $V_{BG}$  and  $V_G$  at  $T=1.5K$  as shown in lower panel of Fig. S2 b. Here  $V_G$  is the graphene gate voltage which is applied directly to the graphene to tune the NW density as shown in the measurement schematic in Fig. S2 a. The black and green dashed lines indicate the trajectories of  $V_{D1}$  and  $V_{D2}$  with changing gate voltages. The arrows in the upper panel indicate that, both  $V_{D1}$  and  $V_{D2}$  of the two plots are essentially same. We observe that, as  $V_G$  increases, the Dirac point shifts towards positive values of  $V_{BG}$ . This is obvious as the graphene channel becomes less electron doped as we apply +ve  $V_G$  and less -ve  $V_{BG}$  gate is required to make the graphene charge neutral. From the 2D plot, we find the slope of  $V_{D1}$  to be close to unity which supports the above argument. In our measurement setup, the graphene and NW are separated by a thin hBN ( $\sim 10nm$ ) flake. So, applying  $V_G$  in graphene induces charge carriers in the NW as well as in graphene region below the NW. Since the electric field generated from the backgate is well-screened by the graphene, NW density is mostly controlled by  $V_G$ , whereas  $V_{BG}$  controls the density of the rest of the graphene channel. As a result, the graphene portion below NW acquires different doping when graphene gate is applied i.e. when  $V_G \neq 0V$  (upper panel of fig. S2(b)) which indicates that the density inhomogeneity of the graphene channel is intrinsically present most likely due to trap charge impurities at the NW-hBN-Graphene structure. As we observe from the 2D plot, the  $V_{D2}$  changes faster than  $V_{D1}$  when  $V_G$  is applied which is evident from the above discussion. We also calculate the slope of  $V_{D2}$  trajectory and find that the capacitance of the graphene gate  $C_G \sim 20 \times C_{BG}$ , where  $C_{BG}$  is the capacitance of the backgate. From this equation, we estimate the thickness of the top hBN to be  $\sim 12 - 15nm$  which is very close to the thickness of the hBN used ( $\sim 10nm$ ). While calculating the  $C_G$ , we have not included the quantum capacitances of the systems.

## SI 4. Modulation in density of states

We generated the density of states (DOS) of graphene using a MATLAB code according to the algorithm mentioned below. Let the dimensions of the graphene sheet be  $(L_X, L_Y)$ , with Area (A) =  $L_X \times L_Y$ . Then the spacing of wave vectors  $(K_X, K_Y)$  will be,  $\Delta K_X = 2\pi/L_X$  and  $\Delta K_Y = 2\pi/L_Y$ . At first we construct a 2D  $K_X$ - $K_Y$  array as shown in fig. S5 a. Then, we calculate the energy corresponding to each K-point using the low energy dispersion relation,  $E = \hbar v_F \sqrt{(K_X^2 + K_Y^2)}$ . Finally, we count the number of K-points ( $\delta N(\epsilon)$ ) for a given energy  $\epsilon$ , which satisfies  $\epsilon - \delta\epsilon < E(K_X, K_Y) < \epsilon + \delta\epsilon$ . Once we have all the above information, the DOS( $\epsilon$ ) is given by,

$$DOS(\epsilon) = 4 \times \frac{\delta N(\epsilon)}{2\delta\epsilon} \times \frac{1}{A}$$

Here, 4 factor in the numerator is the degeneracy of the system i.e. the number of states that can occupy the same K-point.

To incorporate the effect of disorder, we introduced a Gaussian broadening into the system. For this we average the original DOS with an weightage of Gaussian function and the resulting effective DOS ( $DOS'$ ) is given by,

$$DOS'(\epsilon) = \int_{-\delta E}^{\delta E} DOS(\epsilon + x) G(x) dx$$

Where,  $G(x) = \frac{1}{\sqrt{2\pi\delta E_F^2}} e^{\frac{-x^2}{2\delta E_F^2}}$  is the Gaussian function and  $\delta E_F$  is the Fermi energy broadening of the system. Using the above algorithm, we estimate the DOS for two-dimensional graphene with a dimension of  $10\mu\text{m} \times 10\mu\text{m}$  (black curve) as well as of  $10\mu\text{m} \times 0.6\mu\text{m}$  (red curve) as shows in Fig. S5 b.

## SI 5. Cavity strength and Length Scale calculations

**Cavity strength:** In this section we discuss how the cavity strength has been calculated. As discussed before, a cavity is created in graphene in the region beneath the NW in presence of NW's one-dimensional electrostatic potential. From the backgate response of graphene, we observe a second Dirac point  $V_{D2}$  appears at negative gate voltages which suggests existence of more electron like or 'n' type region in the graphene sheet and implicates uneven density profile across the graphene channel. As shown in Fig. 4b (lower panel) of main manuscript, the density mismatch across the graphene sheet leads to misaligned Fermi energies which creates a energy barrier or confinement for the charge carriers. We have estimated the density mismatch from the backgate voltage difference between  $V_{D1}$  and  $V_{D2}$ . To estimate the strength of the energy barrier, we use the linear band dispersion of monolayer graphene  $E_F = \hbar v_F \sqrt{\pi n_G}$  and parabolic band dispersion  $E_F = \frac{\pi \hbar^2 n_G}{2m^*}$  for bilayer graphene with  $m^* \sim 0.03m_0$ , where  $v_F$ ,  $m^*$  and  $m_0$  are the Fermi velocity and the effective mass of carriers in bilayer

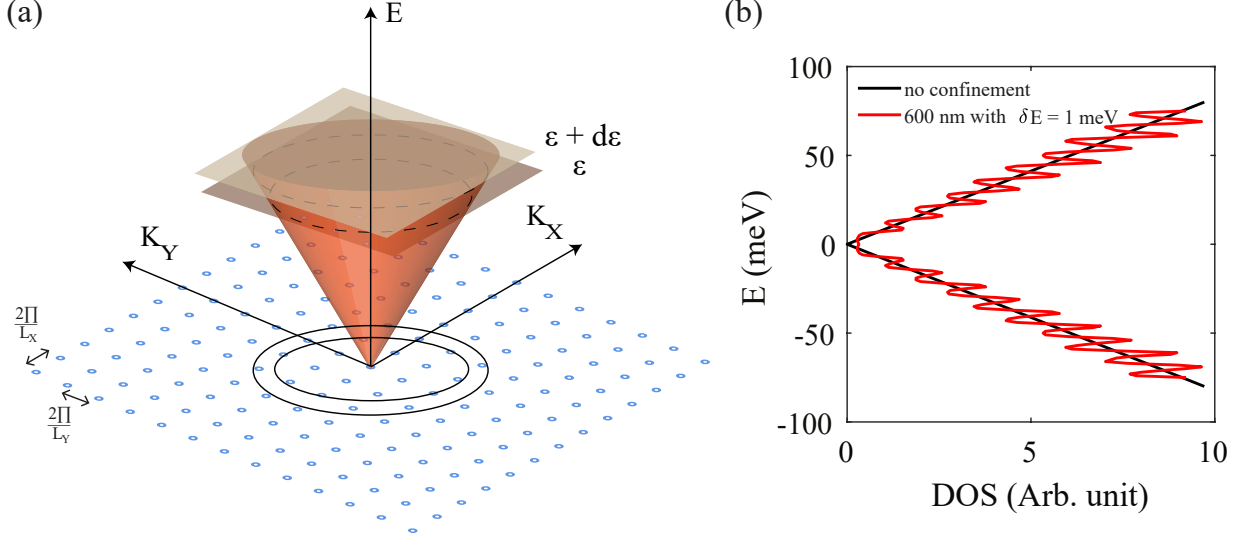

**Figure S5** (a) Reciprocal lattice distribution for samples having dimension  $L_X \times L_Y$  having equal length and for unequal length. (b) Fermi energy plot with density of states (DOS) for graphene having dimension of  $10\mu\text{m} \times 10\mu\text{m}$  (black) and  $10\mu\text{m} \times 0.6\mu\text{m}$  (red) with a Gaussian broadening of  $\delta E = 1$  meV.

graphene and the mass of electron, respectively. For our devices,  $\Delta V_{BG} = V_{D2} - V_{D1} \sim 16V$  and  $\sim 23V$  for MLG and BLG respectively which is equivalent to energy scale of  $\sim 115\text{meV}$  and  $\sim 45\text{meV}$ . The  $R_G$  versus  $E_F$  plots for MLG and BLG devices are shown in Fig. S6 a and b, respectively. The smaller energy barrier in bilayer graphene indicates shallow confinement of charge carriers which explains the absence of oscillations in BLG devices.

**Length Scale calculations:** We also estimate the approximate length scale corresponding to the oscillations observed in MLG devices. As shown in Fig. 3a of main manuscript, the average oscillation period in MLG is  $\delta n \sim 0.8 \times 10^{10}/\text{cm}^2$  which is equivalent to the energy  $\delta E \sim 10\text{meV}$ . The cavity length for a constructive interference is:  $L = p\lambda$ , where  $\lambda$  is the electron wavelength and  $p$  is any positive integer. This equation reduces to  $L = \frac{2\pi\hbar v_F}{\delta E}$  for MLG. For our systems  $\delta E \sim 7 - 10\text{meV}$  which is equivalent to length  $0.6 - 0.4\mu\text{m}$ . This length scale is very similar to the NW channel length in our devices which shows that the confinement barrier is created underneath the NW contacts. To estimate the fluctuation period corresponding to the other dimension (diameter) of the NW, we use  $L \sim 50\text{nm}$  which is equivalent to  $\delta n \sim 1.25 - 5 \times 10^{11}\text{cm}^{-2}$ . Since significant oscillations are not observed among  $\pm 0.5 \times 10^{11}\text{cm}^{-2}$ , we can infer that the confinement or the cavity is formed only along the length of the NW. The cavity is weaker along the diameter, which could be due to shallow confinement arising from the cylindrical shape of the NW.

**Effect of screening:** Now, we will discuss the density dependence of  $V_{TE}$  oscillations. It can be seen in Fig. 3a of the manuscript that the oscillations in  $V_{TE}$  get weaker as  $n_G$  increases. The Fermi energy increases along with  $n_G$ . However, the oscillations in the DOS as a function of energy do not show any decrease with increasing  $E$  in Fig. 4c of the manuscript.

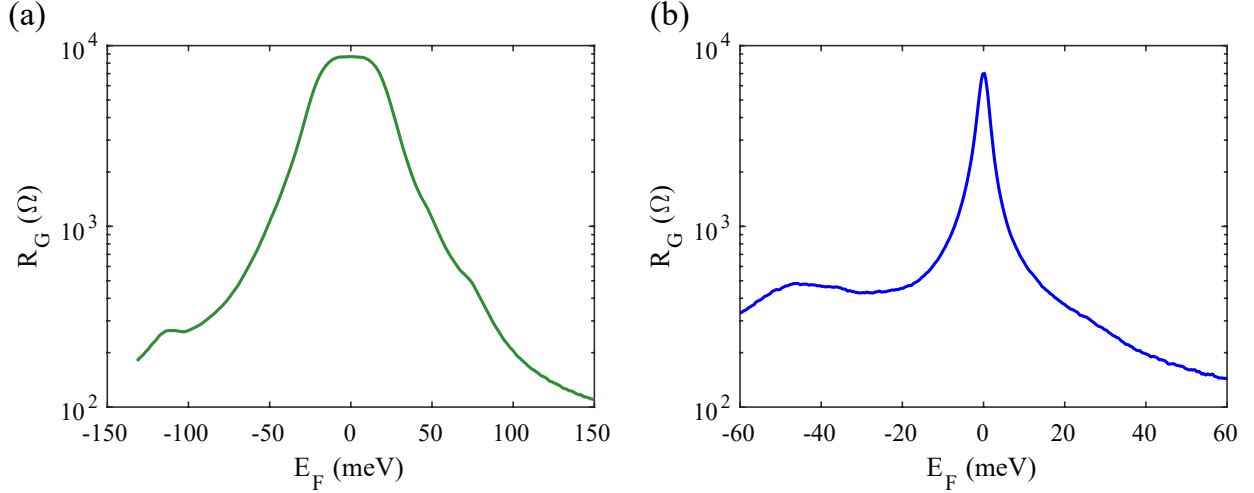

**Figure S6** (a) and (b) are plots of  $R_G$  vs. Fermi energy  $E_F$  for MLG and BLG, respectively. The second peak of  $R_G$  appears around 115 meV and 45 meV for MLG and BLG devices.

The most probable cause for the decrease in oscillations with increasing  $n_G$  is the effect of screening. Note that for MLG, the DOS, in the absence of confinement goes as  $|E|$  and thus increases with increasing  $n_G$ . The cavity potential itself is affected by the ability of the layer to screen since it is induced by the NW on top. Thus, as  $n_G$  increases, so does the amount of screening effectively resulting in a decrease in the strength of the confining potential. Since the oscillations are caused due to the confinement, they too decrease in magnitude with increasing  $n_G$ . The DOS shown in Fig. 4c of the manuscript while correctly showing that oscillations in the DOS exist, does not take this effect of screening at large  $n_G$  into account, since it is difficult to model it accurately. The importance of screening can also be seen from the fact that the estimated cavity potential for MLG is larger than for BLG. In the latter system, the DOS is more or less constant and does not go to zero at the charge neutrality point. Screening in BLG is thus more effective and the potential induced by the NW much weaker.

## SI 6: Thermopower in BLG in presence of magnetic field

Fig. S7 a and b shows plots of  $V_{TE}$  with  $n_G$  for different magnetic fields for MLG and BLG devices respectively. For MLG, the oscillation period increases as B is increased. This indicates the formation of Landau levels (LL) for  $B > 0.1T$  (Fig. 5a of main manuscript). At  $B=0T$ ,  $V_{TE}$  changes sign according to the Seebeck coefficient polarity for the BLG device. In presence of the magnetic field, the thermopower voltage starts to show oscillations which indicate the formation of Landau levels in the BLG also. The energy equivalent to the oscillation frequency for BLG (Fig. 5c of main manuscript) matches with the expected energy gap between LLs for BLG.

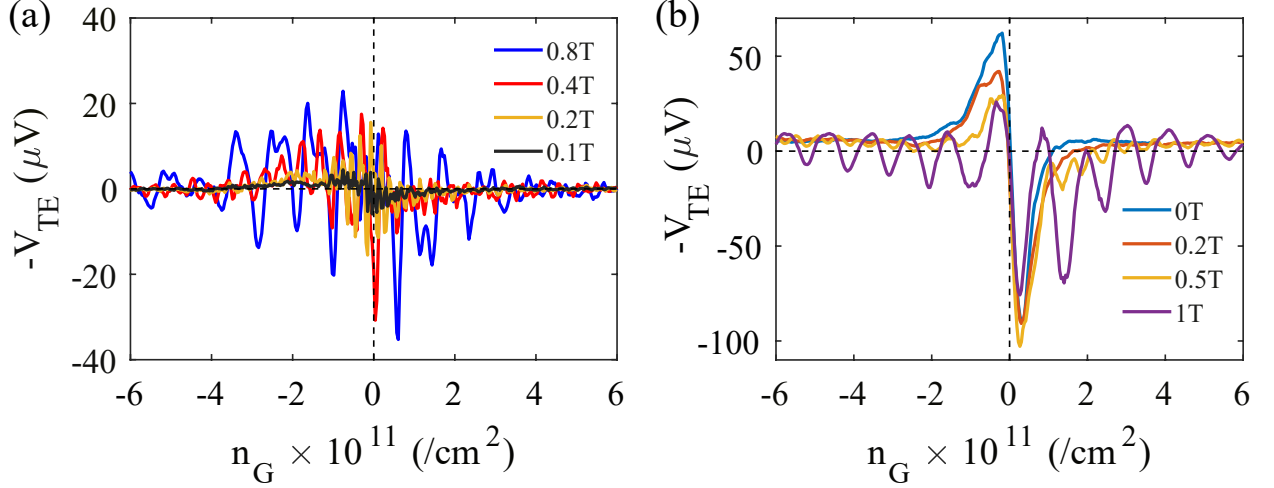

**Figure S7**  $V_{TE}$  plot with  $n_G$  for different magnetic fields at  $T=1.5K$  for MLG (a) and BLG (b) respectively. The vertical and horizontal dashed lines indicate Dirac point and the zero thermopower respectively.

## SI 7: Theoretical Model

To calculate the temperature profile in the graphene layer, we solve the 3D Fourier heat diffusion equation for the multilayer stack. The stack comprises, from top to bottom (thicknesses in parentheses): hBN (10 nm), graphene (0.4 nm), hBN (25 nm), SiO<sub>2</sub> (300 nm), Si (500  $\mu$ m). The stack is heated by an InAs NW placed on top of the top hBN layer, represented by a planar rectangular heat source. We consider three components of this heat source: (1) the NW channel (length = 0.6  $\mu$ m, width = 50 nm), (2) NW underneath the left contact (length = 0.93  $\mu$ m, width = 50 nm), (3) NW underneath the right contact (length = 0.93  $\mu$ m, width = 50 nm). The power dissipated in part (1) is  $P$ , and in parts (2) and (3) is  $f_L P$  and  $f_R P$ , respectively. We calculate the 3D temperature profile induced by each of these heat sources separately, and obtain the total temperature profile by superposition.

### Numerical approach

To calculate the temperature profile created a rectangular surface heat source, we use a closed form analytical solution [6] for the steady-state 3D Fourier diffusion equation:  $\nabla^2 \theta = 0$ , where  $\theta(x, y, z) = T(x, y, z) - T_0$  is the temperature rise above ambient. The simulation cell has dimensions  $L_x$  and  $L_y$  (both taken to be 60  $\mu$ m). The heat source, whose center is at coordinates  $(X_0, Y_0)$ , has dimensions  $H_x$  and  $H_y$  along the x and y directions, respectively. We assume adiabatic boundary conditions on the top and lateral surfaces, and isothermal conditions ( $\theta = 0$ ) at the bottom of the Si substrate. Key equations are reproduced below from Bagnall et al. [6] to aid the reader.

The general solution for the temperature rise at a point located at a depth  $z_j$  within the  $j$ th layer is given by:

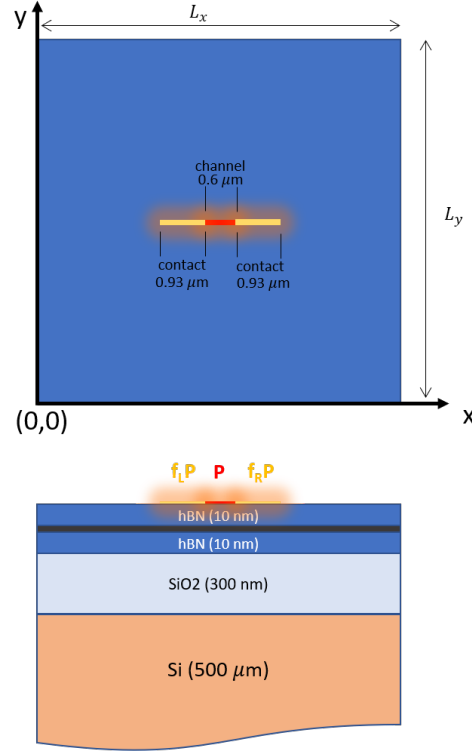

**Figure S8** (Upper panel) Top view of the theoretical set up where the NW is represented by the smaller rectangular region on top of the graphene channel (blue region) having dimension of  $L_x \times L_y$ . Here the yellow and the red portions represents the metal contacts and the channel of the NW respectively. (Lower panel) The side view of the setup showing the multilayer stacking.

$$\begin{aligned}
\theta_j(x, y, z_j) = & A_{0j} + B_{0j}z + \sum_{m=1}^{\infty} \cos(\lambda_m x) [A_{1j} \cosh(\lambda_m z_j) + B_{1j} \sinh(\lambda_m z_j)] \\
& + \sum_{n=1}^{\infty} \cos(\delta_n y) [A_{2j} \cosh(\delta_n z_j) + B_{2j} \sinh(\delta_n z_j)] + \\
& \sum_{m=1}^{\infty} \sum_{n=1}^{\infty} \cos(\lambda_m x) \cos(\delta_n y) [A_{3j} \cosh(\beta_{mn} z_j) + B_{3j} \sinh(\beta_{mn} z_j)]
\end{aligned}$$

where  $\lambda_m = m\pi/L_x$ ,  $\delta_n = n\pi/L_y$  and  $\beta_{mn} = \sqrt{\lambda_m^2 + \delta_n^2}$  are the eigenvalues, collectively denoted  $\gamma_n$ . The Fourier coefficients  $A_{ij}$  and  $B_{ij}$  in the  $j$ th layer are related by the spreading function,  $\phi_j(\gamma_n) = -B_{ij}/A_{ij}$ . Assuming a high heat transfer coefficient at the bottommost surface of the Si substrate (i.e. thermally grounded to ambient), and given that its large thickness,  $\phi_N(\gamma_n) = 1$ . The spreading functions in layers 1 to N-1 are found recursively:

$$\phi_j(\gamma_n) = \frac{\frac{\kappa_j}{\kappa_{j+1}} \tanh(\gamma_n t_j) + \phi_{j+1}(\gamma_n) + \frac{\kappa_j}{G_j} \gamma_n \phi_{j+1}(\gamma_n) \tanh(\gamma_n t_j)}{\frac{\kappa_j}{\kappa_{j+1}} + \phi_{j+1}(\gamma_n) \tanh(\gamma_n t_j) + \frac{\kappa_j}{G_j} \gamma_n \phi_{j+1}(\gamma_n)}$$

where  $\kappa_j$  and  $t_j$  denote the thermal conductivity and thickness of layer  $j$  respectively, and  $G_j$  the thermal boundary conductance between layers  $j$  and  $j+1$ . The zeroth order Fourier coefficients  $A_{0j}$  and  $B_{0j}$  are given by:

$$\begin{aligned}
A_{0j} &= \frac{Q}{L_x L_y} \left( \sum_{l=j}^N \left[ \frac{t_l}{\kappa_l} + \frac{1}{G_l} \right] \right) \\
B_{0j} &= -\frac{Q}{L_x L_y \kappa_j}
\end{aligned}$$

Higher order Fourier coefficients in the top layer,  $A_{i1}$  ( $i = 1, 2, 3$ ) are given by:

$$\begin{aligned}
A_{11} &= \frac{4P \cos(\lambda_m X_0) \sin(\frac{1}{2} \lambda_m H_x)}{L_x L_y H_x \kappa_1 \lambda_m^2 \phi_1(\lambda_m)} \\
A_{21} &= \frac{4P \cos(\delta_n Y_0) \sin(\frac{1}{2} \delta_n H_y)}{L_x L_y H_y \kappa_1 \delta_n^2 \phi_1(\delta_n)} \\
A_{31} &= \frac{16P \cos(\lambda_m X_0) \sin(\frac{1}{2} \lambda_m H_x) \cos(\delta_n Y_0) \sin(\frac{1}{2} \delta_n H_y)}{L_x L_y H_x H_y \kappa_1 \lambda_m \delta_n \beta_{mn} \phi_1(\beta_{mn})}
\end{aligned}$$

Finally, Fourier coefficients in the lower layers are defined using the recursive relation:

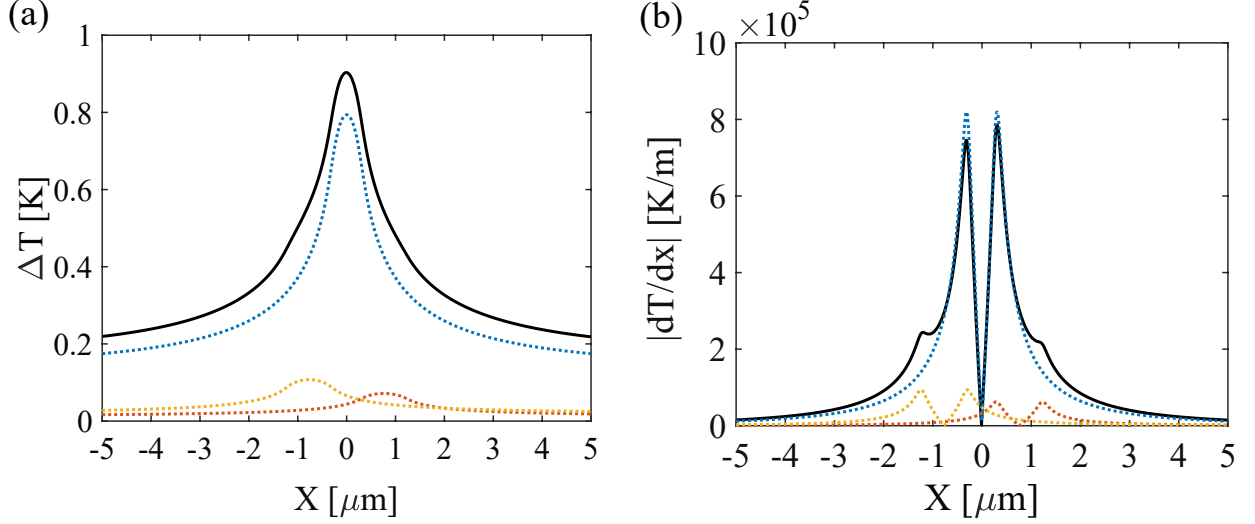

**Figure S9** (a) The temperature rise  $\Delta T$  plotted with position along the  $X$  direction. (b) The absolute value of the temperature gradient  $| \frac{dT}{dX} |$  plotted with position  $X$ . For both the plots, the dashed blue, yellow, and red curves correspond to the individual heating contributions from the NW channel, the left, and right contacts, respectively. The total temperature rise and the temperature gradient are shown by the black curves respectively.

$$A_{ij} = A_{i,j-1} \left[ \frac{\cosh(\gamma_n t_{j-1}) - \phi_{j-1}(\gamma_n) \sinh(\gamma_n t_{j-1})}{\frac{\kappa_j}{G_j} \gamma_n \phi_j(\gamma_n) + 1} \right]$$

Since some of the layers in the stack are thermally anisotropic, we account for this by defining effective isotropic values for thickness and thermal conductivity:  $\kappa_{j,iso} = \sqrt{(\kappa_{j,z} \kappa_{j,xy})}$  and  $t_{j,iso} = t_j / \sqrt{\kappa_{j,z} / \kappa_{j,xy}}$ , where ‘xy’ and ‘z’ refer to in-plane and cross-plane components.

## Thermal parameters

The inputs to this model are the thickness ( $t$ ) and thermal conductivity ( $\kappa$ ) of each layer, and the thermal boundary conductance ( $G$ ) between adjacent layers. Below we describe how these properties are estimated at a base temperature of  $\sim 5$  to  $10$  K, based on prior experiments and calculations. We emphasize that our goal is not to calculate the precise temperature profile, but to obtain a first order estimate of the temperature gradients.

For  $\kappa_{xy}$  of hBN, we refer to previous low T measurements [7] of heat transport in crystallites of diameter  $\sim 1 \mu\text{m}$  and thickness  $\sim 50$ - $100$  nm. At low T, it is reasonable to assume that phonon boundary scattering is specular, and therefore  $\kappa_{xy}$  is thickness-independent. Since the lateral dimensions will limit phonon transport, we must scale  $\kappa_{xy}$  by  $10\times$  to account for the distance between the metal contacts in our devices, viz.  $10 \mu\text{m}$ ; this gives  $\kappa_{xy} \approx 30 \text{ Wm}^{-1}\text{K}^{-1}$  at  $5$  K. We assume that at low T, intrinsic cross-plane transport in hBN is not limiting, but rather governed by interfaces (see below), and take a sufficiently large  $\kappa_z$  so that it does not matter.

For graphene, we first estimate the electronic contribution to  $\kappa_{xy}$  using the Wiedemann Franz law, which was previously shown [8] to be valid below 20 K. Based on the measured electrical conductivity, we estimate this to be at most  $\approx 2 \text{ Wm}^{-1}\text{K}^{-1}$  at highest doping. To estimate the lattice contribution, we refer to first principles calculations [9] for polycrystalline graphene of grain size  $\sim 10 \text{ }\mu\text{m}$ , which gave  $\sim 100 \text{ Wm}^{-1}\text{K}^{-1}$  at 5 K. However, since these calculations were for suspended graphene, we must account for phonon scattering with the substrate. To first order, we assume the same suppression factor as at room temperature [10] and estimate the lattice contribution to be  $\approx 20 \text{ Wm}^{-1}\text{K}^{-1}$ . For  $\text{SiO}_2$  and doped Si, we refer to previous low T measurements and extrapolate where necessary [11, 12];  $\kappa_{\text{SiO}_2} \approx 0.1 \text{ Wm}^{-1}\text{K}^{-1}$ , and  $\kappa_{\text{Si}} \approx 1 \text{ Wm}^{-1}\text{K}^{-1}$ .

Interfaces are known to limit heat transport in vdW heterostructures. For graphene/hBN, we refer to calculations based on non-equilibrium Green's function [13];  $G_{\text{hBN/graphene}} \approx 1 \text{ M Wm}^{-2}\text{K}^{-1}$  at 5 K. The same thermal conductance is assumed for the hBN/ $\text{SiO}_2$  and  $\text{SiO}_2/\text{Si}$  interfaces - they do not significantly affect the temperature profile in graphene.

For the calculations shown in the main text, we take  $P = 1 \text{ }\mu\text{W}$ , and impose an asymmetry in heating at the contacts by assuming  $f_L = 0.15$ ,  $f_R = 0.1$ . The gradient of the temperature profile is non-zero largely within  $\sim \pm 1 \text{ }\mu\text{m}$  of the center as show in Fig. S9. Fig. S9 a shows the plot of calculated temperature rise  $\Delta T$  versus position  $X$  whereas Fig. S9 b shows the temperature gradient plot with  $X$ . Both the plots shows individual contribution from the NW channel, left and right contacts towards the mentioned parameters.

## References

- [1] Novoselov, K. S. *et al.* Electric field effect in atomically thin carbon films. *science* **306**, 666–669 (2004).
- [2] Purdie, D. *et al.* Cleaning interfaces in layered materials heterostructures. *Nature communications* **9**, 5387 (2018).
- [3] Wang, L. *et al.* One-dimensional electrical contact to a two-dimensional material. *Science* **342**, 614–617 (2013).
- [4] Suyatin, D., Thelander, C., Björk, M., Maximov, I. & Samuelson, L. Sulfur passivation for ohmic contact formation to inas nanowires. *Nanotechnology* **18**, 105307 (2007).
- [5] Mitra, R. *et al.* Anomalous coulomb drag between inas nanowire and graphene heterostructures. *Physical Review Letters* **124**, 116803 (2020).
- [6] Bagnall, K. R., Muzychka, Y. S. & Wang, E. N. Analytical solution for temperature rise in complex multilayer structures with discrete heat sources. *IEEE Transactions on Components, Packaging and Manufacturing Technology* **4**, 817–830 (2014).
- [7] Sichel, E., Miller, R., Abrahams, M. & Buiocchi, C. Heat capacity and thermal conductivity of hexagonal pyrolytic boron nitride. *Physical review B* **13**, 4607 (1976).
- [8] Crossno, J. *et al.* Observation of the dirac fluid and the breakdown of the wiedemann-franz law in graphene. *Science* **351**, 1058–1061 (2016).
- [9] Fugallo, G. *et al.* Thermal conductivity of graphene and graphite: collective excitations and mean free paths. *Nano letters* **14**, 6109–6114 (2014).
- [10] Yang, J. *et al.* Thermal conductance imaging of graphene contacts. *Journal of Applied Physics* **116**, 023515 (2014).
- [11] Dutta, M. & Jackson, H. E. Low-temperature thermal conductivity of amorphous silica. *Physical Review B* **24**, 2139 (1981).
- [12] Asheghi, M., Kurabayashi, K., Kasnavi, R. & Goodson, K. Thermal conduction in doped single-crystal silicon films. *Journal of applied physics* **91**, 5079–5088 (2002).
- [13] Liu, Y. *et al.* Thermal conductance of the 2d mos 2/h-bn and graphene/h-bn interfaces. *Scientific reports* **7**, 43886 (2017).
